# Supplementary material for: Exploring Italian sentence embeddings properties through multi-tasking
Source: arXiv:2409.06622 source file (2024-11-29)
Supplement: Supplementary file 1 [file appendix-archspecs.tex]

\section{Architectural Specifications}
\label{arch-specs}

All systems used a learning rate of 0.001 and Adam optimizer, and batch size 100. The training was done for 120 epochs. The experiments were run on an HP PAIR Workstation Z4 G4 MT, with435 an Intel Xeon W-2255 processor, 64G RAM, and a MSI GeForce RTX 3090 VENTUS 3X OC 24G GDDR6X GPU.

We tested BERT sentence embeddings with baseline CNN and FFNN baseline architectures. \cite{devlin-etal-2019-bert}. The sentence embeddings are the encoding of the [CLS] token on the last layer of the model.

The FFNN receives the input as a concatenation of sentence embeddings in a sequence, with a size of 7 * 768. This input is then processed through 3 fully connected layers, which progressively compress the input size (7 * 768 $\rightarrow{layer 1}$ 3.5 * 768 $\rightarrow{layer 2}$ 3.5 * 768 $\rightarrow{layer 3}$ 768) to obtain the size of a sentence representation. The FFNN's interconnected layers enable it to capture patterns that are distributed throughout the entire input vector.

The CNN takes as input an array of embeddings with a size of (7 x 768). This input undergoes three consecutive layers of 2-dimensional convolutions, where each convolutional layer uses a kernel size of (3x3) and a stride of 1, without dilation. The resulting output from the convolutional process is then passed through a fully connected layer, which compresses it to the size of the sentence representation (768). By using a kernel size of (3x3), stride=1, and no dilation, this configuration emphasizes the detection of localized patterns within the sentence sequence array. 

%If the encoding of noun phrases (NPs) and verb grammatical numbers is concentrated in specific regions of the sentence representation, this architecture has the capability to identify those patterns within the sequence.

Both networks produce the same output, which is a vector representing the sentence embedding of the correct answer. The objective of learning is to maximize the probability of selecting the correct answer from a set of candidate answers. To achieve this, we employ the max-margin loss function, considering that the incorrect answers in the answer set are intentionally designed to have minimal differences from the correct answer. This loss function combines the distances between the predicted answer and both the correct and incorrect answers. Initially, we calculate a score for each candidate answer's embedding $e_i$ in the answer set $\mathcal{A}$ with respect to the predicted sentence embedding $e_{pred}$. This score is determined by the cosine of the angle between the respective vectors:

\[
  score(e_i, e_{pred}) = cos(e_i,e_{pred})
\]

The loss function incorporates the max-margin concept, taking into account the difference between the score of the correct answer $e_c$ and each of the incorrect answers $e_i$:

\[
loss_a = \sum_{e_i} [1 - score(e_c, e_{pred}) + score(e_i,e_{pred})]^{+}
\]

During prediction, the answer with the highest score value from the candidate set is selected as the correct answer.
